# Supplementary material for: Fine-Grained Analysis of Catastrophic Forgetting in Continual Learning via Algorithmic Stability
Source: arXiv:2610.31551 source file (2026-10-22)
Supplement: Supplementary file 1 [file Joint_Generalization_Gaps.tex]

\section{Joint Analysis of Generalization Gaps}\label{Sec: proof of joint analysis}
In this section, we prove Theorems~\ref{Thm: joint bound convex} and~\ref{Thm: joint bound non-convex}. We use the sampling and domain conditions stated in Section~\ref{Sec: algorithmic-stability}. All sums over SGD steps use $t=0,\ldots,N-1$, and an empty product equals one.

\subsection{Coupled Trajectories and the Joint Generalization Gap}
Fix $i\in[T-1]$ and two datasets $S_{1:T}$ and $S_{1:T}'$ that differ only at position $k$ of task $i$. Run SGD on these datasets using the same initialization and the same sampled indices. Write $w_{\tau,t}$ and $w_{\tau,t}'$ for the resulting trajectories, and let $w_\tau=w_{\tau,N}$ and $w_\tau'=w_{\tau,N}'$. The two trajectories coincide before task $i$, so $w_{i,0}=w_{i,0}'$. Since the loss is differentiable and $L$-Lipschitz on the open domain $\Omega$, its gradient satisfies $\|\nabla f(w;z)\|\le L$ for every $w\in\Omega$ and $z\in\mathcal Z$. Indeed, the directional derivative in any unit direction is bounded in absolute value by $L$.

We first relate the joint generalization gap to the effect of replacing one training example. For each $k\in[n]$, draw $\widetilde z_{i,k}\sim\mathcal D_i$ independently of the datasets and algorithmic randomness, and let $S_{1:T}^{(i,k)}$ be obtained by replacing $z_{i,k}$ with $\widetilde z_{i,k}$. For $\tau\in\{i,T\}$, exchangeability of $z_{i,k}$ and $\widetilde z_{i,k}$ gives
\begin{equation}\label{Eqn: joint ghost exchange}
\begin{aligned}
&\mathbb E_{S_{1:T},\mathcal A}f(w_\tau(S_{1:T});z_{i,k})=\mathbb E_{S_{1:T},\widetilde z_{i,k},\mathcal A}
f(w_\tau(S_{1:T}^{(i,k)});\widetilde z_{i,k}).
\end{aligned}
\end{equation}
Here, the same realization of the algorithmic randomness is used in both runs. The independent replacement sample is included in the expectation on the right-hand side. Applying Equation~\eqref{Eqn: joint ghost exchange} at both training stages yields
\begin{equation}\label{Eqn: joint ghost representation}
\begin{aligned}
&\mathbb E_{S_{1:T},\mathcal A}\big[
R_{\mathcal D_i}(w_T)-R_{S_i}(w_T)-R_{\mathcal D_i}(w_i)+R_{S_i}(w_i)\big]\\
&=\frac1n\sum_{k=1}^n
\mathbb E_{S_{1:T},\widetilde z_{i,k},\mathcal A}\big[
f(w_T;\widetilde z_{i,k})-f(w_i;\widetilde z_{i,k})\\
&\hspace{5mm}-f(w_T';\widetilde z_{i,k})
+f(w_i';\widetilde z_{i,k})\big],
\end{aligned}
\end{equation}
where the primed iterates in each summand are computed from $S_{1:T}^{(i,k)}$. Consequently, a uniform upper bound on
\begin{equation}\label{Eqn: joint coupled increment}
\mathbb E_{\mathcal A}\big|
f(w_T;z)-f(w_i;z)-f(w_T';z)+f(w_i';z)
\big|
\end{equation}
also bounds $\epsilon^{\mathrm{joint}}_{T,i}$. To apply this statement, we condition on the datasets and the replacement sample in Equation~\eqref{Eqn: joint ghost representation}, so that the evaluation point is fixed, and then average over them.

The following inequality controls the four-point expression in Equation~\eqref{Eqn: joint coupled increment}. Convexity of $\Omega$ ensures that the segments joining the paired iterates remain in the domain. For each fixed $z$, the fundamental theorem of calculus gives, for $\tau\in\{i,T\}$,
\begin{equation*}
\begin{aligned}
&f(w_\tau;z)-f(w_\tau';z)\\
&=\int_0^1\big\langle
\nabla f(w_\tau'+\theta(w_\tau-w_\tau');z),
w_\tau-w_\tau'\big\rangle\,d\theta.
\end{aligned}
\end{equation*}
Subtracting the two identities, using the gradient bound on the difference of the displacement vectors, and using smoothness on the difference of the gradients, we obtain
\begin{equation}\label{Eqn: joint four point}
\begin{aligned}
&\big|f(w_T;z)-f(w_i;z)-f(w_T';z)+f(w_i';z)\big|\\
&\le L\big\|(w_T-w_T')-(w_i-w_i')\big\|\\
&\quad+\beta\|w_i-w_i'\|\int_0^1
\big\|(1-\theta)(w_T'-w_i')+\theta(w_T-w_i)\big\|\,d\theta\\
&\le L\big\|(w_T-w_T')-(w_i-w_i')\big\|\\
&\quad+\frac\beta2\big(\|w_T'-w_i'\|+\|w_T-w_i\|\big)
\|w_i-w_i'\|.
\end{aligned}
\end{equation}
This inequality uses the first derivative and its Lipschitz continuity. It holds in both the convex and non-convex settings. In addition, bounded gradients give the following pathwise bounds for the two trajectories:
\begin{equation}\label{Eqn: joint trajectory displacement}
\begin{aligned}
\|w_T-w_i\|&\le L\sum_{\tau=i+1}^T\sum_{t=0}^{N-1}\eta_{\tau,t},\\
\|w_T'-w_i'\|&\le L\sum_{\tau=i+1}^T\sum_{t=0}^{N-1}\eta_{\tau,t}.
\end{aligned}
\end{equation}

\subsection{Proof of Theorem~\ref{Thm: joint bound convex}}\label{Sec: proof of joint bound convex}
\begin{proof}
Under convexity, smoothness, and $0\le\eta_{\tau,t}\le2/\beta$, the gradient update using any fixed example is non-expansive by Lemma~\ref{Lem: f property}. During task $i$, the coupled runs select the replaced position with probability $1/n$, independently of the previous updates. If the selected position differs from the replaced position, non-expansivity bounds the next distance by the current distance. Otherwise, the two gradient norms are each at most $L$, and the next distance is at most the current distance plus $2L\eta_{i,t}$. Hence,
\begin{equation*}
\begin{aligned}
&\mathbb E_{\mathcal A}\|w_{i,t+1}-w_{i,t+1}'\|\le\mathbb E_{\mathcal A}\|w_{i,t}-w_{i,t}'\|
+\frac{2L\eta_{i,t}}n.
\end{aligned}
\end{equation*}
Since $w_{i,0}=w_{i,0}'$, unrolling the recursion gives
\begin{equation}\label{Eqn: joint convex local distance}
\mathbb E_{\mathcal A}\|w_i-w_i'\|
\le\frac{2L}{n}\sum_{t=0}^{N-1}\eta_{i,t}.
\end{equation}
All subsequent tasks use identical datasets and sampled indices in the two runs. Applying non-expansivity to these shared updates therefore gives, for every $\tau>i$ and $t\in\{0,\ldots,N\}$,
\begin{equation}\label{Eqn: joint convex future distance}
\|w_{\tau,t}-w_{\tau,t}'\|\le\|w_i-w_i'\|.
\end{equation}
We also need to control the change in the displacement vector. Summing the differences of the future SGD updates, and then using smoothness and Equation~\eqref{Eqn: joint convex future distance}, yields
\begin{equation}\label{Eqn: joint convex vector change}
\begin{aligned}
&\big\|(w_T-w_T')-(w_i-w_i')\big\|\\
&\le\beta\sum_{\tau=i+1}^T\sum_{t=0}^{N-1}
\eta_{\tau,t}\|w_{\tau,t}-w_{\tau,t}'\|\\
&\le\beta\left(\sum_{\tau=i+1}^T\sum_{t=0}^{N-1}\eta_{\tau,t}\right)
\|w_i-w_i'\|.
\end{aligned}
\end{equation}
Substituting Equations~\eqref{Eqn: joint trajectory displacement} and~\eqref{Eqn: joint convex vector change} into Equation~\eqref{Eqn: joint four point}, we obtain
\begin{equation*}
\begin{aligned}
&\big|f(w_T;z)-f(w_i;z)-f(w_T';z)+f(w_i';z)\big|\\
&\le2\beta L\left(\sum_{\tau=i+1}^T\sum_{t=0}^{N-1}\eta_{\tau,t}\right)
\|w_i-w_i'\|.
\end{aligned}
\end{equation*}
Taking the expectation over the algorithmic randomness and applying Equation~\eqref{Eqn: joint convex local distance} gives
\begin{equation}\label{Eqn: joint convex cancellation proof}
\begin{aligned}
&\mathbb E_{\mathcal A}\big|f(w_T;z)-f(w_i;z)
-f(w_T';z)+f(w_i';z)\big|\\
&\le\frac{4\beta L^2}{n}
\left(\sum_{t=0}^{N-1}\eta_{i,t}\right)
\left(\sum_{\tau=i+1}^T\sum_{t=0}^{N-1}\eta_{\tau,t}\right).
\end{aligned}
\end{equation}
Alternatively, applying the Lipschitz property at each endpoint and then Equation~\eqref{Eqn: joint convex future distance} gives
\begin{equation*}
\begin{aligned}
&\big|f(w_T;z)-f(w_i;z)-f(w_T';z)+f(w_i';z)\big|\\
&\le L\big(\|w_T-w_T'\|+\|w_i-w_i'\|\big)
\le2L\|w_i-w_i'\|.
\end{aligned}
\end{equation*}
Combining its expectation with Equation~\eqref{Eqn: joint convex cancellation proof}, and using Equation~\eqref{Eqn: joint ghost representation}, proves
\begin{equation}\label{Eqn: joint convex appendix bound}
\begin{aligned}
\epsilon^{\mathrm{joint}}_{T,i}
&\le\frac{4L^2}{n}\left(\sum_{t=0}^{N-1}\eta_{i,t}\right)\times\min\left\{
\beta\sum_{\tau=i+1}^T\sum_{t=0}^{N-1}\eta_{\tau,t},\,1\right\}.
\end{aligned}
\end{equation}
When $\beta=0$, each sample gradient is constant on $\Omega$. Shared updates then preserve the displacement vector, and Equation~\eqref{Eqn: joint four point} gives a zero four-point difference. Thus, the same conclusion holds without a step-size restriction in this case.
\end{proof}

\subsection{Proof of Theorem~\ref{Thm: joint bound non-convex}}\label{Sec: proof of joint bound non-convex}
\begin{proof}
For a shared example, smoothness gives
\begin{equation*}
\|w_{i,t+1}-w_{i,t+1}'\|
\le(1+\beta\eta_{i,t})\|w_{i,t}-w_{i,t}'\|.
\end{equation*}
When the replaced position is selected, bounded gradients instead give
\begin{equation*}
\|w_{i,t+1}-w_{i,t+1}'\|
\le\|w_{i,t}-w_{i,t}'\|+2L\eta_{i,t}.
\end{equation*}
Conditioning on the previous updates, the two cases occur with probabilities $1-1/n$ and $1/n$, respectively. Averaging them yields
\begin{equation*}
\begin{aligned}
&\mathbb E_{\mathcal A}\|w_{i,t+1}-w_{i,t+1}'\|\\
&\le\left(1+\left(1-\frac1n\right)\beta\eta_{i,t}\right)
\mathbb E_{\mathcal A}\|w_{i,t}-w_{i,t}'\|
+\frac{2L\eta_{i,t}}n.
\end{aligned}
\end{equation*}
Unrolling this recursion from the common initialization of task $i$ gives
\begin{equation}\label{Eqn: joint nonconvex local distance}
\begin{aligned}
&\mathbb E_{\mathcal A}\|w_i-w_i'\|\\
&\le\frac{2L}{n}\sum_{t=0}^{N-1}\eta_{i,t}
\prod_{s=t+1}^{N-1}
\left(1+\left(1-\frac1n\right)\beta\eta_{i,s}\right).
\end{aligned}
\end{equation}
After task $i$, every update is shared. Repeatedly applying the smoothness bound gives, for $\tau>i$ and $t\in\{0,\ldots,N\}$,
\begin{equation}\label{Eqn: joint nonconvex future distance}
\begin{aligned}
&\|w_{\tau,t}-w_{\tau,t}'\|\\
&\le\left[\prod_{\kappa=i+1}^{\tau-1}\prod_{s=0}^{N-1}
(1+\beta\eta_{\kappa,s})\right]
\left[\prod_{s=0}^{t-1}(1+\beta\eta_{\tau,s})\right]
\|w_i-w_i'\|.
\end{aligned}
\end{equation}
To control the change in the displacement vector, we sum the gradient differences along the future updates. Equation~\eqref{Eqn: joint nonconvex future distance} then gives
\begin{equation}\label{Eqn: joint nonconvex vector change}
\begin{aligned}
&\big\|(w_T-w_T')-(w_i-w_i')\big\|\\
&\le\beta\sum_{\tau=i+1}^T\sum_{t=0}^{N-1}
\eta_{\tau,t}\|w_{\tau,t}-w_{\tau,t}'\|\\
&\le\Bigg[\sum_{\tau=i+1}^T\sum_{t=0}^{N-1}\beta\eta_{\tau,t}
\prod_{\kappa=i+1}^{\tau-1}\prod_{s=0}^{N-1}(1+\beta\eta_{\kappa,s})\\
&\hspace{5mm}\times\prod_{s=0}^{t-1}(1+\beta\eta_{\tau,s})\Bigg]
\|w_i-w_i'\|\\
&=\left[\prod_{\tau=i+1}^T\prod_{t=0}^{N-1}(1+\beta\eta_{\tau,t})-1\right]
\|w_i-w_i'\|.
\end{aligned}
\end{equation}
The last equality follows by expanding the product in chronological order. Each summand is the difference between the products immediately after and before one update, so the sum telescopes.

Substituting Equations~\eqref{Eqn: joint trajectory displacement} and~\eqref{Eqn: joint nonconvex vector change} into Equation~\eqref{Eqn: joint four point} yields
\begin{equation}\label{Eqn: joint nonconvex four point bound}
\begin{aligned}
&\big|f(w_T;z)-f(w_i;z)-f(w_T';z)+f(w_i';z)\big|\\
&\le L\Bigg[
\prod_{\tau=i+1}^T\prod_{t=0}^{N-1}(1+\beta\eta_{\tau,t})-1\\
&\hspace{19mm}+\beta\sum_{\tau=i+1}^T\sum_{t=0}^{N-1}\eta_{\tau,t}
\Bigg]\|w_i-w_i'\|.
\end{aligned}
\end{equation}
We can also bound the two endpoints separately. The Lipschitz property and Equation~\eqref{Eqn: joint nonconvex future distance} imply
\begin{equation*}
\begin{aligned}
&\big|f(w_T;z)-f(w_i;z)-f(w_T';z)+f(w_i';z)\big|\\
&\le L\left[\prod_{\tau=i+1}^T\prod_{t=0}^{N-1}(1+\beta\eta_{\tau,t})+1\right]
\|w_i-w_i'\|.
\end{aligned}
\end{equation*}
Taking the expectation over the algorithmic randomness in both bounds, substituting Equation~\eqref{Eqn: joint nonconvex local distance}, and applying Equation~\eqref{Eqn: joint ghost representation} gives
\begin{equation}\label{Eqn: joint nonconvex appendix bound}
\begin{aligned}
&\epsilon^{\mathrm{joint}}_{T,i}\\
&\le\frac{2L^2}{n}\Bigg[\sum_{t=0}^{N-1}\eta_{i,t}
\prod_{s=t+1}^{N-1}\left(1+\left(1-\frac1n\right)\beta\eta_{i,s}\right)\Bigg]\\
&\quad\times\min\Bigg\{
\prod_{\tau=i+1}^T\prod_{t=0}^{N-1}(1+\beta\eta_{\tau,t})-1+\beta\sum_{\tau=i+1}^T\sum_{t=0}^{N-1}\eta_{\tau,t},\\
&\hspace{5mm}\prod_{\tau=i+1}^T\prod_{t=0}^{N-1}(1+\beta\eta_{\tau,t})+1
\Bigg\}.
\end{aligned}
\end{equation}
All factors are well defined for $n=1$, zero step sizes, and $\beta=0$. In particular, the first term inside the minimum is zero when there are no subsequent updates or when $\beta=0$.
\end{proof}

\subsection{Learning Rate Schedules and Comparison with Separate Bounds}
We next substitute the three learning rate schedules into the preceding results. These expressions retain the finite sums and products, including the first task under continuously decaying learning rates.

For convex losses, Equation~\eqref{Eqn: joint convex appendix bound} gives the following bounds. Under constant learning rates $\eta_{\tau,t}=c$,
\begin{equation}\label{Eqn: joint convex constant appendix}
\epsilon^{\mathrm{joint}}_{T,i}
\le\frac{4cL^2N}{n}\min\{c\beta N(T-i),1\}.
\end{equation}
Under intra-task decaying learning rates $\eta_{\tau,t}=c/(t+1)$,
\begin{equation}\label{Eqn: joint convex ID appendix}
\begin{aligned}
\epsilon^{\mathrm{joint}}_{T,i}
&\le\frac{4cL^2}{n}\left(\sum_{t=0}^{N-1}\frac1{t+1}\right)\\
&\quad\times\min\left\{c\beta(T-i)\sum_{t=0}^{N-1}\frac1{t+1},1\right\}.
\end{aligned}
\end{equation}
Under continuously decaying learning rates $\eta_{\tau,t}=c/((\tau-1)N+t+1)$,
\begin{equation}\label{Eqn: joint convex CD appendix}
\begin{aligned}
\epsilon^{\mathrm{joint}}_{T,i}
&\le\frac{4cL^2}{n}\left(\sum_{t=0}^{N-1}\frac1{(i-1)N+t+1}\right)\\
&\quad\times\min\left\{c\beta\sum_{\tau=i+1}^T\sum_{t=0}^{N-1}
\frac1{(\tau-1)N+t+1},1\right\}.
\end{aligned}
\end{equation}
For $\beta>0$, the condition $c\le2/\beta$ ensures the required step-size restriction for all three schedules and all historical tasks. For a fixed $i$, the continuously decaying schedule also permits $c\le2((i-1)N+1)/\beta$, because only task $i$ and its subsequent tasks require non-expansive updates.

For non-convex losses, substituting constant learning rates into Equation~\eqref{Eqn: joint nonconvex appendix bound} gives
\begin{equation}\label{Eqn: joint nonconvex constant appendix}
\begin{aligned}
\epsilon^{\mathrm{joint}}_{T,i}
&\le\frac{2cL^2}{n}\Bigg[\sum_{t=0}^{N-1}
\left(1+\left(1-\frac1n\right)c\beta\right)^{N-1-t}\Bigg]\\
&\quad\times\min\Big\{
(1+c\beta)^{N(T-i)}-1+c\beta N(T-i),\\
&\hspace{26mm}(1+c\beta)^{N(T-i)}+1\Big\}.
\end{aligned}
\end{equation}
Under intra-task decaying learning rates, the corresponding bound is
\begin{equation}\label{Eqn: joint nonconvex ID appendix}
\begin{aligned}
\epsilon^{\mathrm{joint}}_{T,i}
&\le\frac{2cL^2}{n}\Bigg[\sum_{t=0}^{N-1}\frac1{t+1}
\prod_{s=t+1}^{N-1}\left(1+\left(1-\frac1n\right)\frac{c\beta}{s+1}\right)\Bigg]\\
&\quad\times\min\Bigg\{
\left[\prod_{t=0}^{N-1}\left(1+\frac{c\beta}{t+1}\right)\right]^{T-i}-1\\
&\hspace{26mm}+c\beta(T-i)\sum_{t=0}^{N-1}\frac1{t+1},\\
&\hspace{26mm}\left[\prod_{t=0}^{N-1}\left(1+\frac{c\beta}{t+1}\right)\right]^{T-i}+1
\Bigg\}.
\end{aligned}
\end{equation}
Under continuously decaying learning rates, we obtain
\begin{equation}\label{Eqn: joint nonconvex CD appendix}
\begin{aligned}
\epsilon^{\mathrm{joint}}_{T,i}
&\le\frac{2cL^2}{n}\Bigg[\sum_{t=0}^{N-1}\frac1{(i-1)N+t+1}\\
&\hspace{10mm}\times\prod_{s=t+1}^{N-1}
\left(1+\left(1-\frac1n\right)\frac{c\beta}{(i-1)N+s+1}\right)\Bigg]\\
&\quad\times\min\Bigg\{
\prod_{\tau=i+1}^T\prod_{t=0}^{N-1}
\left(1+\frac{c\beta}{(\tau-1)N+t+1}\right)-1\\
&\hspace{20mm}+c\beta\sum_{\tau=i+1}^T\sum_{t=0}^{N-1}
\frac1{(\tau-1)N+t+1},\\
&\hspace{12mm}\prod_{\tau=i+1}^T\prod_{t=0}^{N-1}
\left(1+\frac{c\beta}{(\tau-1)N+t+1}\right)+1\Bigg\}.
\end{aligned}
\end{equation}

We now compare joint and separate analyses using the same trajectory estimates. In the convex setting, applying Equation~\eqref{Eqn: joint convex local distance} at the two endpoints gives the separate bound $4L^2\sum_{t=0}^{N-1}\eta_{i,t}/n$. When this quantity is positive, the joint bound is strictly smaller if and only if
\begin{equation}\label{Eqn: joint convex strict comparison appendix}
\beta\sum_{\tau=i+1}^T\sum_{t=0}^{N-1}\eta_{\tau,t}<1.
\end{equation}
In the non-convex setting, Equations~\eqref{Eqn: joint nonconvex local distance} and~\eqref{Eqn: joint nonconvex future distance} give the separate bound
\begin{equation}\label{Eqn: joint nonconvex separate comparator}
\begin{aligned}
&\frac{2L^2}{n}\Bigg[\sum_{t=0}^{N-1}\eta_{i,t}
\prod_{s=t+1}^{N-1}\left(1+\left(1-\frac1n\right)\beta\eta_{i,s}\right)\Bigg]\\
&\qquad\times\left[\prod_{\tau=i+1}^T\prod_{t=0}^{N-1}(1+\beta\eta_{\tau,t})+1\right].
\end{aligned}
\end{equation}
When the factor outside the brackets on the second line is positive, Equation~\eqref{Eqn: joint nonconvex appendix bound} is strictly smaller than Equation~\eqref{Eqn: joint nonconvex separate comparator} if and only if
\begin{equation}\label{Eqn: joint nonconvex strict comparison appendix}
\beta\sum_{\tau=i+1}^T\sum_{t=0}^{N-1}\eta_{\tau,t}<2.
\end{equation}
These comparisons follow by subtracting the two future-update factors. For constant, intra-task decaying, and continuously decaying learning rates, the left-hand sides of Equations~\eqref{Eqn: joint convex strict comparison appendix} and~\eqref{Eqn: joint nonconvex strict comparison appendix} are, respectively,
\begin{equation*}
\begin{aligned}
&c\beta N(T-i),\\
&c\beta(T-i)\sum_{t=0}^{N-1}\frac1{t+1},\\
&c\beta\sum_{\tau=i+1}^T\sum_{t=0}^{N-1}\frac1{(\tau-1)N+t+1}.
\end{aligned}
\end{equation*}
Thus, the improvement depends on the cumulative learning rate after task $i$. The comparisons concern the stated upper bounds and do not require the two generalization gaps to have any prescribed signs. The non-convex comparison uses the separate bound in Equation~\eqref{Eqn: joint nonconvex separate comparator}; a separate estimate obtained by optimizing a burn-in time must be compared with the joint bound through its own expression.

If the loss additionally belongs to $[0,1]$, each generalization gap lies in $[-1,1]$, so $\epsilon^{\mathrm{joint}}_{T,i}\le2$. This bound can be combined with the preceding results by taking the minimum. It is a bound on the joint generalization term, whereas the forgetting measure itself belongs to $[-1,1]$ under the same bounded-loss condition.
